# Supplementary material for: Transfer Learning in Automated Gamma Spectral Identification
Source: arXiv:2003.10524 source file (2020-03-23)
Supplement: Supplementary file 1 [file appendix_TL.tex]

\subsection{A. Temperature} \label{temp}
The best tuning of the temperature parameter is an area of active research.  For the purpose of this work a judgement of the best temperature parameter for each architecture was done by examining the levels of separation by different classes in the softened softmax distibution over a validation set from the modeled data Fig~\ref{??????}.
If more labeled data were available

\subsection{B. Binning Schema} \label{binning}

APPENDIX
\begin{itemize}
	\item my temperature figures
	\item 
	
\end{itemize}
